# Supplementary material for: Prometheus: Inducing Fine-grained Evaluation Capability in Language Models
Source: arXiv:2310.08491 source file (2024-03-09)
Supplement: Supplementary file 1 [file code.tex]

\begin{figure*}[t!]
\centering
    \includegraphics[width=0.8\linewidth]{figures/resources/code.pdf}
    \caption{Feedback generated by GPT-4 and Code-Llama trained on the \textsc{Feedback Collection}.}
    \label{figure:code}
\end{figure*}
