# Supplementary material for: Prometheus: Inducing Fine-grained Evaluation Capability in Language Models
Source: arXiv:2310.08491 source file (2024-03-09)
Supplement: Supplementary file 2 [file feedback_collection_taxonomy.tex]

\begin{figure*}[t!]
\centering
    \includegraphics[width=0.99\linewidth]{figures/resources/feedback_collection_taxonomy.pdf}
    \caption{The keywords of the score rubric included in the \textsc{Feedback Collection}.}
    \label{figure:feedback_collection_taxonomy}
\end{figure*}
