# Supplementary material for: Prometheus: Inducing Fine-grained Evaluation Capability in Language Models
Source: arXiv:2310.08491 source file (2024-03-09)
Supplement: Supplementary file 6 [file math.tex]

\begin{figure*}[t!]
\centering
    \includegraphics[width=0.9\linewidth]{figures/resources/math.pdf}
    \caption{Math example of a feedback generated by GPT-4 and Code-Llama 13B trained on the \textsc{Feedback Collection}.}
    \label{figure:math}
\end{figure*}
