# Supplementary material for: Prometheus: Inducing Fine-grained Evaluation Capability in Language Models
Source: arXiv:2310.08491 source file (2024-03-09)
Supplement: Supplementary file 7 [file model-bias-mtbench.tex]

\begin{figure*}[t!]
\centering
    \includegraphics[width=0.9\linewidth]{figures/resources/model_vs_score_gpt4_prometheus_only_percentage_corrected_bar_mt_bench_eval.pdf}
    \caption{}
    \label{figure:model-bias-mtbench}
\end{figure*}
