# Supplementary material for: Prometheus: Inducing Fine-grained Evaluation Capability in Language Models
Source: arXiv:2310.08491 source file (2024-03-09)
Supplement: Supplementary file 9 [file human_eval_feedback_length_diff.tex]

\begin{figure*}[t!]
\centering
    \includegraphics[width=0.8\linewidth]{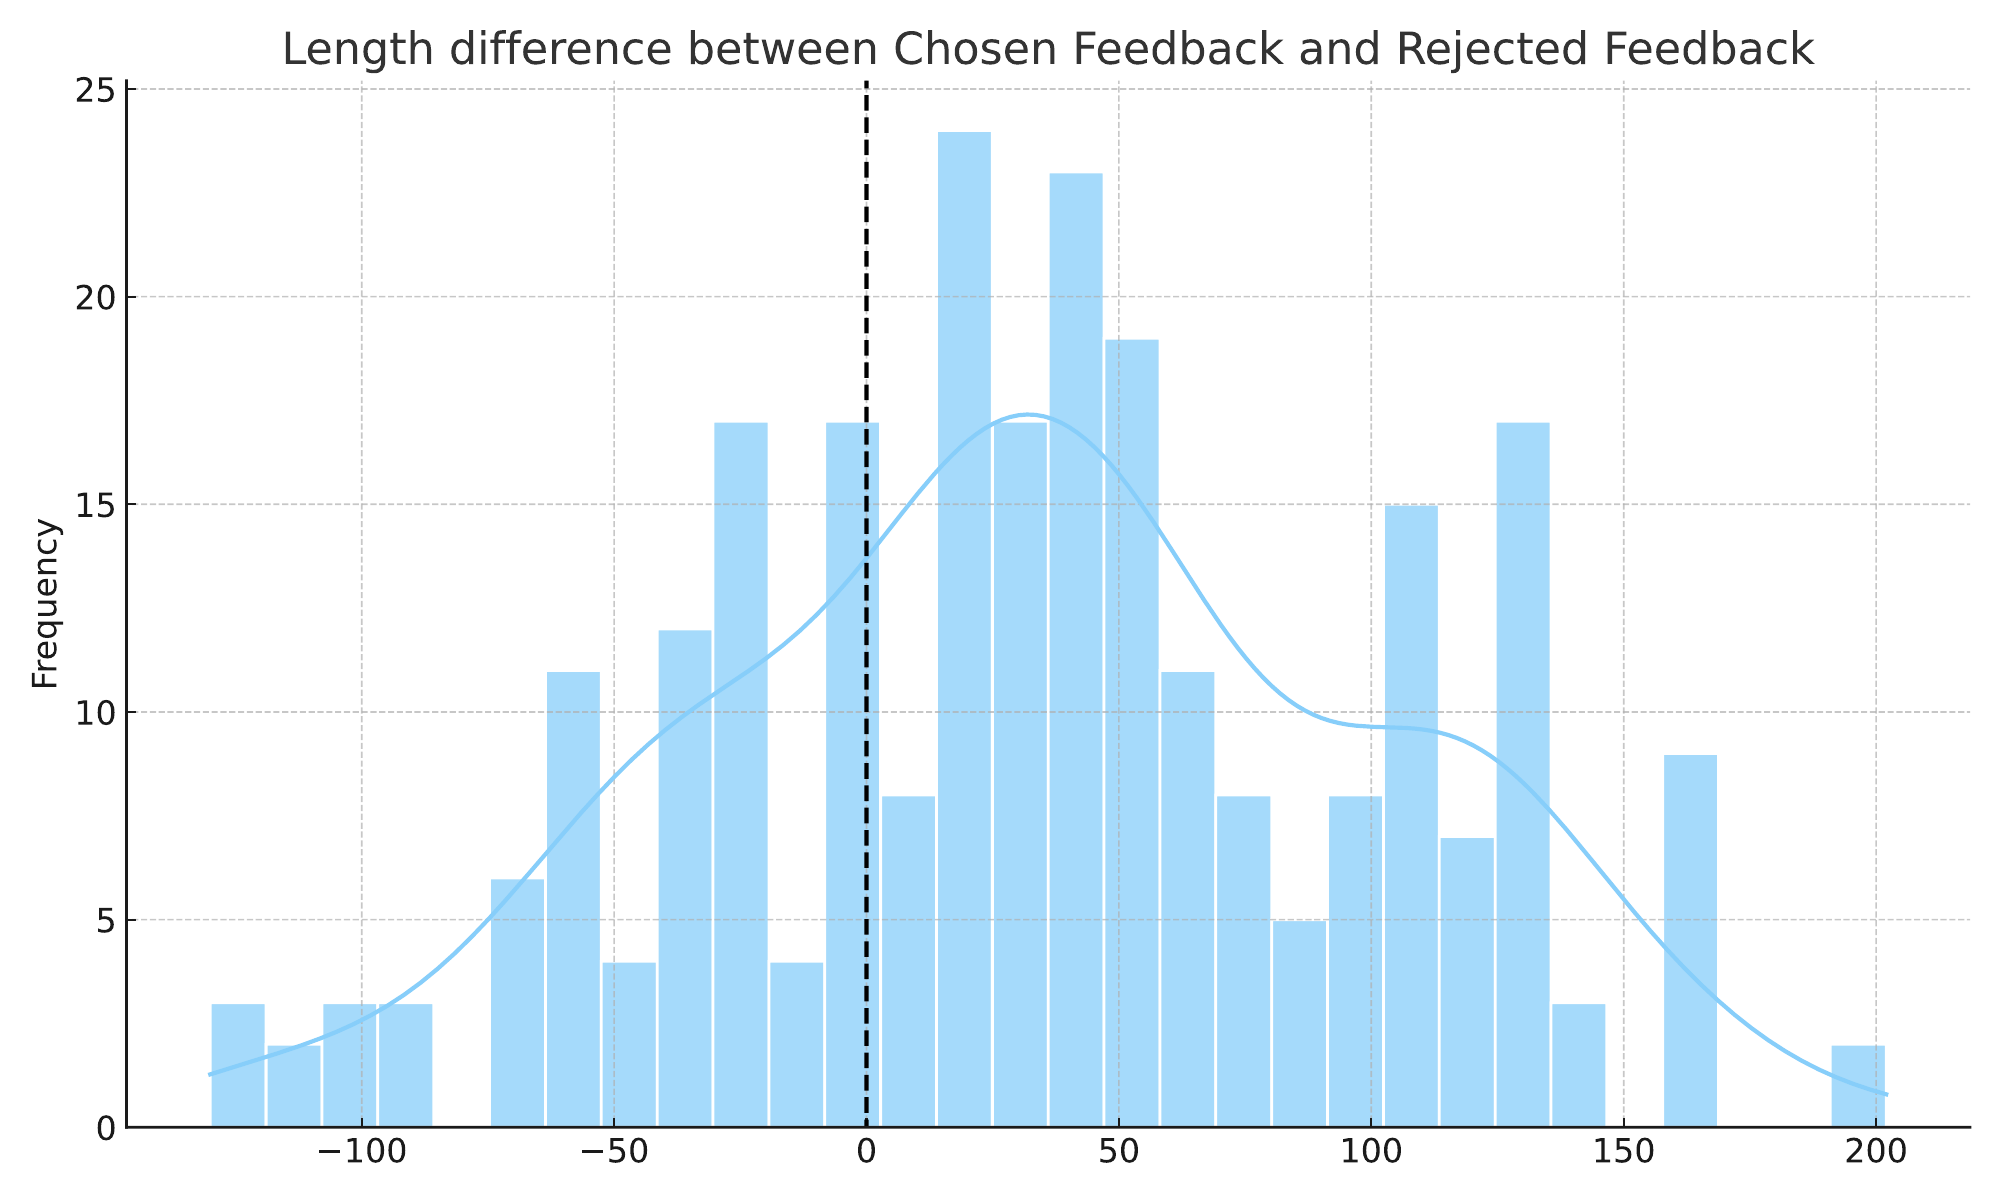}
    \caption{The length difference distribution between the feedback that was chosen over the feedback that was rejected during human evaluation (GPT-4 vs Prometheus).}
    \label{figure:human_eval_feedback_length_diff}
\end{figure*}
